# Supplementary material for: Putative spin liquid in the triangle-based iridate Ba$_3$IrTi$_2$O$_9$
Source: arXiv:1707.03140 source file (2017-07-11)
Supplement: Supplementary file 1 [file supple.pdf]

# Supplementary Material for

# Putative spin liquid in the triangle-based iridate $Ba_3IrTi_2O_9$

W.-J. Lee†,[1] S.-H. Do†,[1] Sungwon Yoon,[2] S. Lee,[1] Y.S. Choi,[1] D.J. Jang,[3] M. Brando,[3] M. Lee,[4] E. S. Choi,[4] S. Ji,[5] Z. H. Jang,[6] B. J. Suh,[2] and K.-Y. Choi[1,*]

[1]*Department of Physics, Chung-Ang University, Seoul 156-756, Republic of Korea*

[2]*Department of Physics, The Catholic University of Korea, Bucheon 420-743, Republic of Korea*

[3]*Max Planck Institute for Chemical Physics of Solids Dresden, Germany*

[4]*National High Magnetic Field Laboratory, Florida State University, Tallahassee, FL 32310, USA*

[5]*Max Planck POSTECH/Korea Research Initiative, Pohang 790-784, Republic of Korea*

[6]*Department of Physics, Kookmin University, Seoul 136-702, Republic of Korea*

(Dated: July 8, 2017)

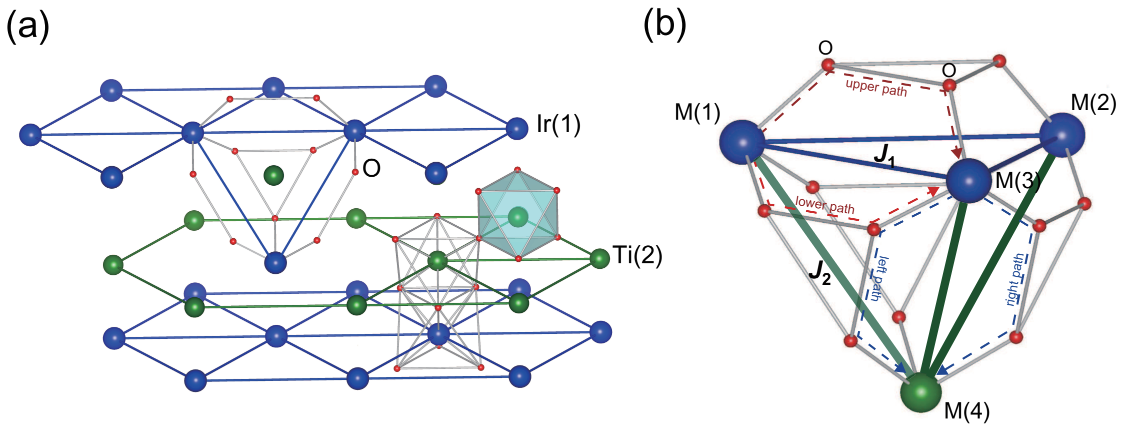


FIG. 1: (a) Crystal structure of $Ba_3IrTi_2O_9$. The $Ir^{4+}$ spins are arranged to form a triangular lattice in the *ab* plane. The blue and green balls represent the iridium and titanium atoms, respectively. The barium atoms are omitted for clarity. A site disorder between $Ti^{4+}$ and $Ir^{4+}$ mainly occurring in the $Ir(1)Ti(2)O_9$ dimers creates a new exchange path, thereby a tetrahdron is derived from the original triangular lattice. (b) A tetrahedron comprising the super-superexchange interaction $J_1$ involving $Ir^{4+}$ spins in the *ab* plane (blue lines) and $J_2$ involving $Ir^{4+}$ spins in the Ir(1) and the Ti(2) layers (green lines).

### A. X-ray powder diffraction of $Ba_3IrTi_2O_9$

$Ba_3IrTi_2O_9$ consists of layers of the structural $Ir(1)Ti(2)O_9$ dimers made of face-sharing octahedra linked by corner-sharing to $Ti(3)O_6$ octahedron layers along the *c* axis as sketched in Fig. 1(a). The $Ir(1)Ti(2)O_9$ dimers (2b site) are separated by the Ti(3) layer (2a site). In the 6H-B structure of $Ba_3IrTi_2O_9$, there is a definite stacking sequence -$Ti^{4+}$(3)-$Ti^{4+}$(2)=$Ir^{4+}$(1)-$Ti^{4+}$(3)-$Ti^{4+}$(2)=$Ir^{4+}$(1) where the "-" sign represents a corner sharing between layers, and the "=" sign represents a face sharing. This renders the $Ir^{4+}$ cations to form an edge-sharing triangular lattice in the *ab* plane. However, it turned out that the $Ba_3MTi_2O_9$ (M=Ru, Ir) compounds are vulnerable to $M^{4+}/Ti^{4+}$ cation disorders of the face sharing octahedra because their ionic radii are similar with the same valence state. In the presence of the cation disorders, the original triangular lattice is depleted, while its edge-sharing connectivity will be no longer maintained.

To clarify the influence of the disorders on magnetic properties, the site occupation of the Ir/Ru and Ti atoms should be first quantified. We address this issue by carrying out x-ray powder diffraction measurements of $Ba_3IrTi_2O_9$ using the PANalytical Empyrean diffrac-

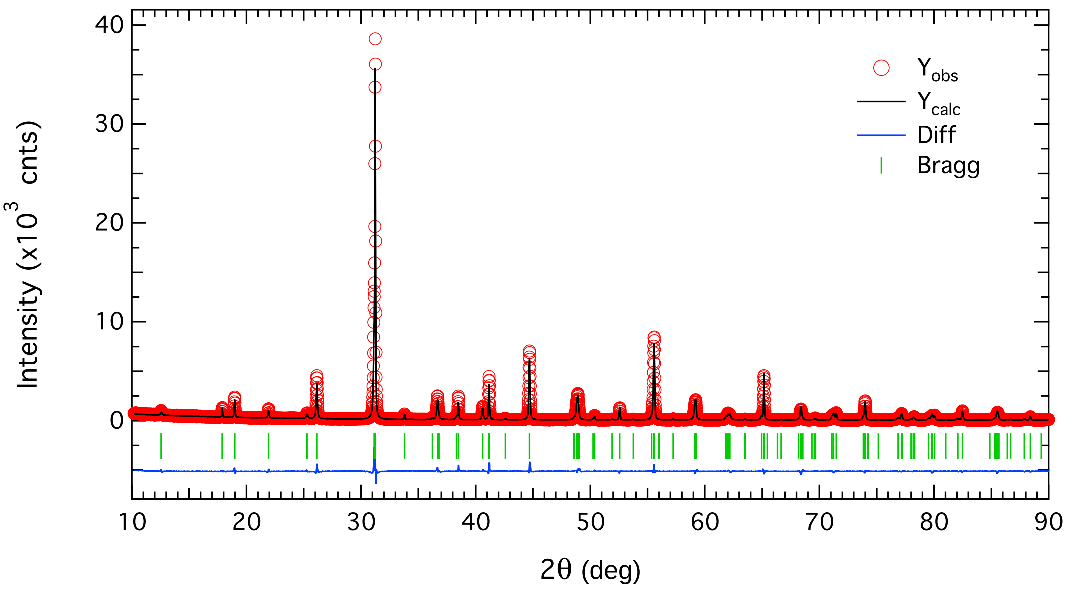


FIG. 2: X-ray powder diffraction data of $Ba_3IrTi_2O_9$ taken at room temperature. The red circles are the experimental data and the black line represents the calculated intensity obtained from the Rietveld refinement. The green bars represent Bragg peak positions and the blue line indicates the difference between the experimental and Rietveld refined intensities.

tometer with Cu $K_\alpha$ radiation ($\lambda$ = 1.54182 Å). No trace of impurity phases could be detected. The Rietveld refinement was made using the FULLPROF program, allowing determining a space group symmetry and an amount of the disorders.

Figure 2 displays the x-ray powder diffraction pattern recorded at room temperature. The XRD patterns of $Ba_3IrTi_2O_9$ can be indexed within the hexagonal structure $P6_3mc$, consistent with the previously reported structure of $Ba_3IrTi_2O_9$ [1]. The goodness of the Rietveld refinement is given by the following parameters; $R_p$=9.39 %, $R_{wp}$=16.9 %, and $\chi^2 = 4.34$. The refinement results of the site occupation are listed in Table I. We find that the Ir(1) 2b sites contain 61.4 % $Ir^{4+}$ and 39.(4) % nonmagnetic $Ti^{4+}$ ions. In the Ti(2) 2b site we found a 42 % site sharing between $Ti^{4+}$ and $Ir^{4+}$. This is in stark contrast to a small 5 % site sharing of $Ti^{4+}$ ions with $Ir^{4+}$ ones in the Ti(3) 2a site. This is explained by the crystal-chemical considerations that the structural dimers of the same Ti-Ti ions are energetically not favorable because an electrostatic repulsion between a pair of $Ti^{4+}$ cations is stronger than that between the $Ti^{4+}$-$Ir^{4+}$ cations. Noteworthy is that 39 % of the cation disorders are close to 33 %, leading to a 1/3 depletion of the triangular network. This

TABLE I: Crystal structure parameters of $Ba_3IrTi_2O_9$ determined by refining the data shown Fig. 1 using the program FULLPROF.

$Ba_3IrTi_2O_9$ at room temperature, $P6_3mc$,

$a = b = 5.7216(1)$ Å, $c = 14.0775(2)$Å, $\alpha = \beta = 90°$, $\gamma = 120°$

$\chi^2 = 4.34$, $R_p = 9.39$ %, $R_{wp} = 12.2$ %

| Atom($W$) | $x$ | $y$ | $z$ | Occup. |
|---|---|---|---|---|
| Ba(1) (2$a$) | 0 | 0 | 0.5 | 1 |
| Ba(2) (2$b$) | 1/3 | 2/3 | 0.8353(5) | 1 |
| Ba(3) (2$b$) | 1/3 | 2/3 | 0.1475(4) | 1 |
| Ti(1) (2$b$) | 1/3 | 2/3 | 0.3985(6) | 0.39(4) |
| Ir(1) (2$b$) | 1/3 | 2/3 | 0.3985(6) | 0.61(4) |
| Ti(2) (2$b$) | 1/3 | 2/3 | 0.5853(7) | 0.58(2) |
| Ir(2) (2$b$) | 1/3 | 2/3 | 0.5853(7) | 0.42(2) |
| Ti(3) (2$a$) | 0 | 0 | 0.2455(14) | 0.95(1) |
| Ir(3) (2$a$) | 0 | 0 | 0.2455(14) | 0.05(1) |
| O(1) (6$c$) | 0.8293(15) | -0.8293(15) | 0.8336(13) | 1 |
| O(2) (6$c$) | 0.4877(18) | -0.4877(18) | 0.5057(17) | 1 |
| O(3) (6$c$) | 0.1532(22) | -0.1532(22) | 0.6716(12) | 1 |

dilution of the edge-shared triangle lattice is anticipated to create 33 % orphan spins, leading to a paramagnetic state at low temperatures. As discussed below, we find no experimental signatures of a large amount of free or weakly interacting spins. Rather, the $Ir^{4+}$ spins residing in the Ti(2) 2b site are strongly exchange coupled to the $Ir^{4+}$ spins in the original triangular lattice. A similar amount of the site disorders is present in $Ba_3RuTi_2O_9$ [2], suggesting that $S = 1$ $Ba_3RuTi_2O_9$ and $J_{\text{eff}} = 1/2$ $Ba_3IrTi_2O_9$ share the same spin topology with a different spin number and distinct spin-orbit coupling.

### B. Exchange paths

In the absence of the site disorders between $Ti^{4+}$ and $Ir^{4+}$, the Ir atoms form a ideal triangular lattice. Due to a 39 % site sharing of $Ir^{4+}$ with $Ti^{4+}$, however, roughly 1/3

TABLE II: List of distances and angles of two different exchange paths forming a tetrahdron.

| Exchange path | | Distance (Å) | | | Angle (degree) | |
|---|---|---|---|---|---|---|
| M(i) - O - O - M(j) | | M(i)-O | O-O | O-M(j) | ∠(M(i)-O-O) | ∠(O-O-M(j)) |
| M(1)-O-O-M(2) | upper path | 2.13571 | 3.05629 | 2.13571 | 128.6074 | 128.6018 |
| | lower path | 1.96632 | 2.76344 | 1.96632 | 138.7828 | 138.7722 |
| M(1)-O-O-M(3) | upper path | 2.13571 | 3.05629 | 2.13571 | 128.6019 | 128.6073 |
| | lower path | 1.96632 | 2.76344 | 1.96632 | 138.7723 | 138.7827 |
| M(2)-O-O-M(3) | upper path | 2.13571 | 3.05629 | 2.13571 | 128.6074 | 128.6019 |
| | lower path | 1.96632 | 2.76344 | 1.96632 | 138.7827 | 138.7722 |
| M(1)-O-O-M(4) | left path | 1.96632 | 3.05629 | 2.02805 | 130.9633 | 133.1137 |
| | right path | 1.96632 | 2.75837 | 2.02805 | 130.9541 | 133.1229 |
| M(2)-O-O-M(4) | left path | 1.96632 | 3.05629 | 2.02804 | 130.9633 | 133.1137 |
| | right path | 1.96632 | 3.05629 | 2.02804 | 130.9541 | 133.1228 |
| M(3)-O-O-M(4) | left path | 1.96632 | 3.05629 | 2.02804 | 130.9540 | 133.1229 |
| | right path | 1.96632 | 3.05629 | 2.02805 | 130.9632 | 133.1136 |

of the $Ir^{4+}$ spins occupy the Ti(2) site. This modifies the original spin topology because the $Ir^{4+}$ spins are exchange coupled along the out-of-plane direction in addition to the in-plane one. In search of all possible exchange paths, we identified the two leading super-superexchange couplings involving Ir-O-O-Ir paths as sketched in Fig. 1(b). We remark that (i) the super-super exchange interactions are not small at all due to the $\sigma$ bonding of O 2p-2p hybridization, and (ii) there is no magnetic dimer because the face sharing octahedra are mostly occupied by couples of $Ir^{4+}/Ti^{4+}$ cations, but not by $Ir^{4+}/Ir^{4+}$ nor $Ti^{4+}/Ti^{4+}$ couples. The strength of the superexchange interactions is determined by the geometrical parameters, that is, a distance and angle of their exchange paths. The in-plane $J_1$ is mediated by the two different exchange paths Ir-O-O-Ir: (i) the upper path with the Ir-O distance 2.1357 Å, the O-O distance 3.0562 Å, and the Ir-O-O angle 128.60° and (ii) the lower path with the Ir-O distance 1.9663 Å, the O-O distance 2.7634 Å, and the Ir-O-O angle 138.77°. The out-of-plane $J_2$ is bridged by the two identical exchange paths with the Ir-O distance 1.9663 Å, the O-O distance 3.0562 Å, the O-Ti/Ir distance 2.0280 Å, the Ir-O-O angle 130.95° and the O-O-Ti/Ir angle 133.12°. From the similar distances and angles

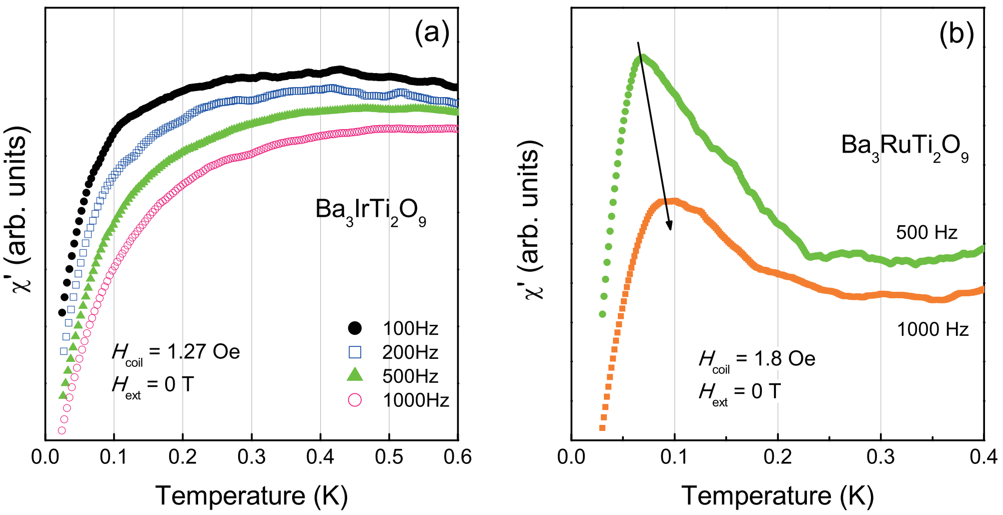


FIG. 3: Real part of the ac susceptibility for $Ba_3IrTi_2O_9$ and $Ba_3RuTi_2O_9$ as a function of temperature (0.02-0.6 K) at four different frequencies.

of the in-plane and out-of-plane Ir-O-O-Ir pathways, we infer that $J_1$ and $J_2$ have an almost equivalent exchange interaction. Based on this consideration, we conclude that the basic building block of $Ba_3IrTi_2O_9$ is given by a 1/4-depleted tetrahedron with nearly identical nearest-neighbor interactions, $J_1 \approx J_2$, rather than by alternating arrays of 1/3- and 2/3-depleted triangular layers along the $c$ axis. Taken together, the $Ir^{4+}$ ions on the decimated 2D tetraheral lattice generate a new frustrated spin motif consisting of both corner- and edge-sharing triangles.

### C. ac susceptibility

The ac susceptibility data were taken with zero external field and ac field of $H = 1.27 - 1.8$ Oe at four different frequencies at $f = 100$, 200, 500, and 1000 Hz using a home-made susceptometer at National High Magnetic Field Lab. An oscillating field of $H = 0.8$ and 1.3 Oe for the Ir and Ru compounds, respectively, was applied with the zero DC magnetic field. The data of $Ba_3RuTi_2O_9$ at 100 and 200 Hz are omitted due to their large noise.

Fig. 3 shows the real part of the ac susceptibility as a function of temperature and frequency. As the temperature is lowered from $T = 0.6$ K, $\chi'(T)$ of $Ba_3IrTi_2O_9$ decreases without showing any sharp peak and frequency dependence. Clearly, this excludes the occurrence of a magnetic order or spin freezing within the precision of our instruments.

In $Ba_3IrTi_2O_9$, the spins are dynamically fluctuating. In contrast, $Ba_3RuTi_2O_9$ displays a maximum at $T = 67$ mK, which shifts to higher temperature with increasing frequency. Such a shift is typical either for an insulating spin-glass or the presence of slow dynamics. However, the absence of an apparent heat capacity anomaly and the persisting spin dynamics seen by $\mu$SR suggests that only a fraction of the spins participate in this glassy phase for $Ba_3RuTi_2O_9$.

**References**

* kchoi@cau.ac.kr

[1] T. Dey, A. V. Mahajan, P. Khuntia, M. Baenitz, B. Koteswararao, and F. C. Chou, Spin-liquid behavior in $J_{eff} = 1/2$ triangular lattice compound $Ba_3IrTi_2O_9$, Phys. Rev. B **86**, 140405(R) (2012).

[2] G. Radtke, C. Maunders, A. Saul, S. Lazar, H. J. Whitfield, J. Etheridge, and G. A. Botton, Phys. Rev. B **81**, 085112 (2010).
